# Supplementary material for: The Impact of Generative Artificial Intelligence on Market Equilibrium: Evidence from a Natural Experiment
Source: arXiv:2311.07071 source file (2024-10-10)
Supplement: Supplementary file 1 [file appendix.tex]

\newpage
\begin{figure}[h]
\centering
\includegraphics[width=0.7\textwidth]{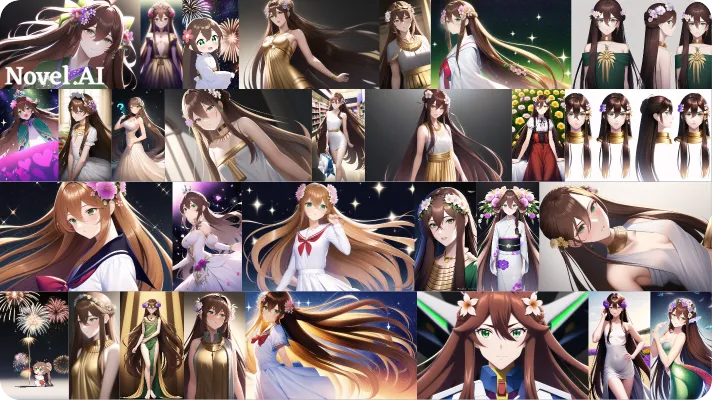}
% \vspace*{-3mm}
\caption{An illustration of the style and quality of NovelAI's AI-generated images.}
\label{fig:novelai}
\vspace*{+10mm}
\end{figure}

\leftline{\Large \textbf{Appendix}}
\section{Robustness Checks}

\subsection{Parallel Trend Assumption} \label{app:parallel}
The parallel trend assumption is justified in the main body of this paper through visual inspection, which demonstrates that the treated and untreated markets exhibited similar trends prior to the leak. This section presents two statistical tests conducted to further verify the parallel trend assumption.
% We justify the parallel trend assumption in the main body of this paper by visual inspection, which shows that the treated and untreated markets were trending similarly before the leak. In this section, we further conduct two statistical tests to verify the parallel trend assumption.

Each order on the focal platform is randomly assigned a number as its ID. We construct a data sample where orders are aggregated according to the last digit of their ID. This results in both the "tachie" and "wallpaper" markets having ten time series in terms of market equilibrium, which facilitates the following statistical tests with more data points.

\subsubsection{Event Study}
We estimate the dynamic treatment effects using the event study specification. Specifically, we estimate the following form:
\begin{equation} \label{equation:main}
y_{it}=\alpha_i +\delta_t + \sum_{j=-L}^{-1} \beta_j\cdot treated_i lead_j + \sum_{k=1}^{R} \beta_k\cdot treated_i lag_k + \varepsilon_{it}
\end{equation}
where $lead_j$ and $lag_k$ are dummy variables, representing $j$ periods before or $k$ periods after a reference period. The reference period was established as the final month that was not affected by the data leak. Given that the leak occurred in October, the last unaffected month was September for order volume and August for price and revenue. This is because consumers can still adjust the prices of orders created in September in response to generative AI.

Figure~\ref{fig:event} illustrates the dynamic treatment effect plots of generative AI on market equilibrium. No clear pre-trend differences between the market equilibrium outcomes of treated and control units are observed. In addition, after the NovelAI leak, the price decreased and the volume and revenue increased significantly, providing compelling support for the parallel trends assumption.

\begin{figure}[h!]
\centering
\includegraphics[width=\textwidth]{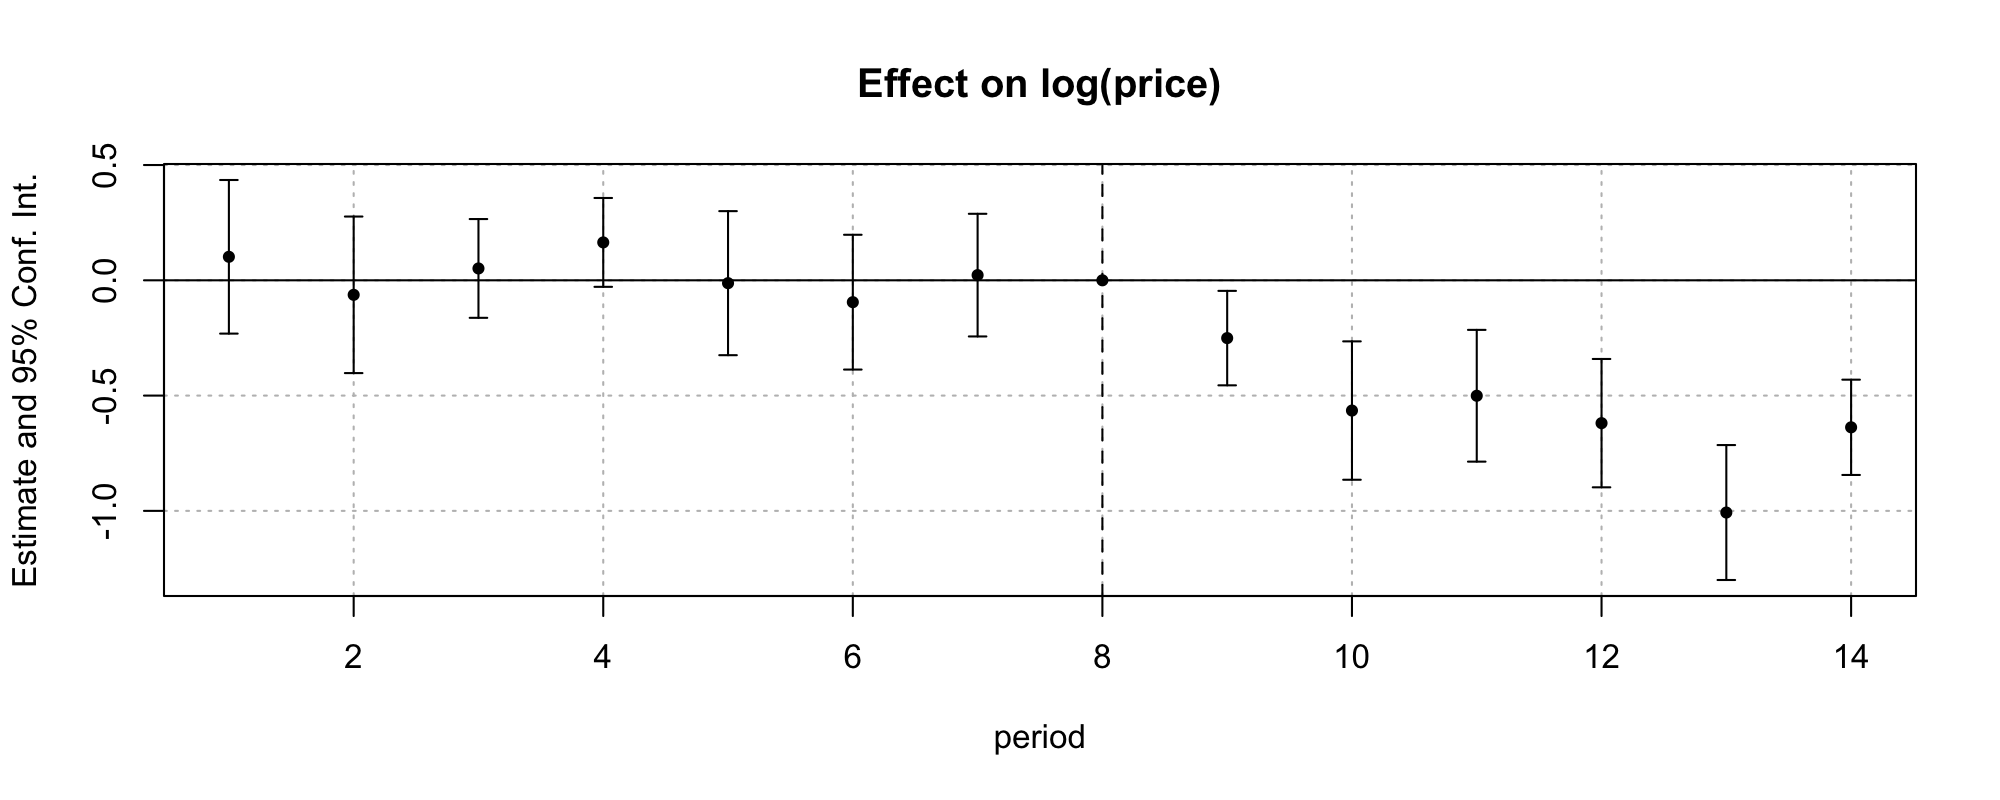}
\includegraphics[width=\textwidth]{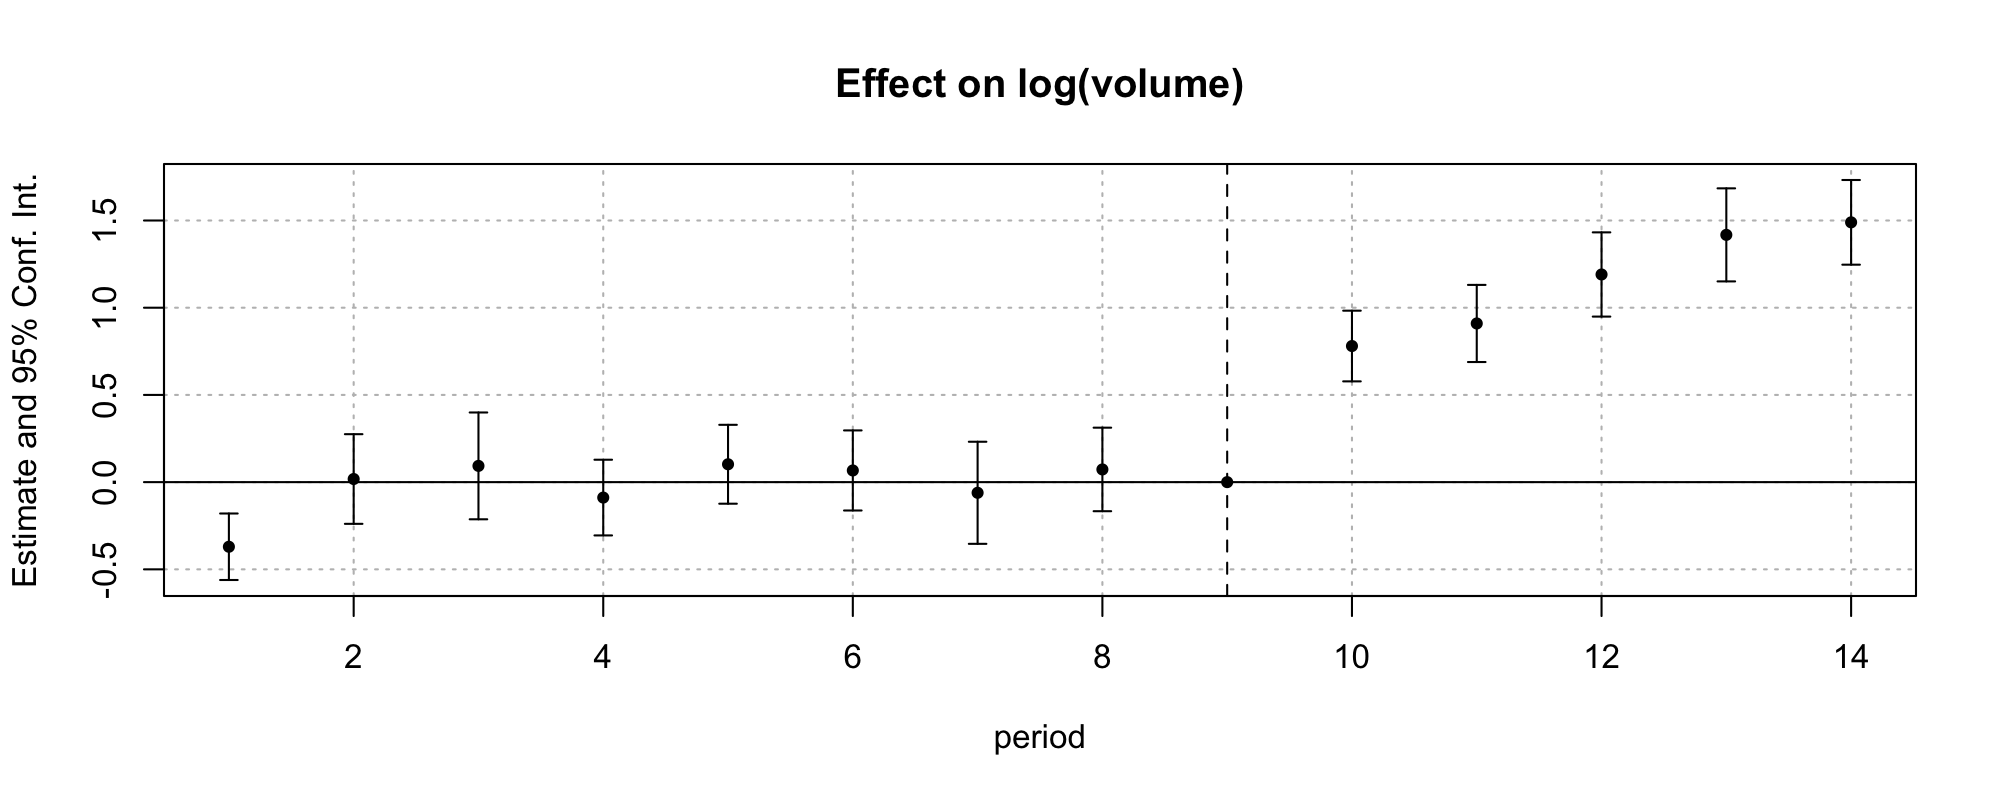}
\includegraphics[width=\textwidth]{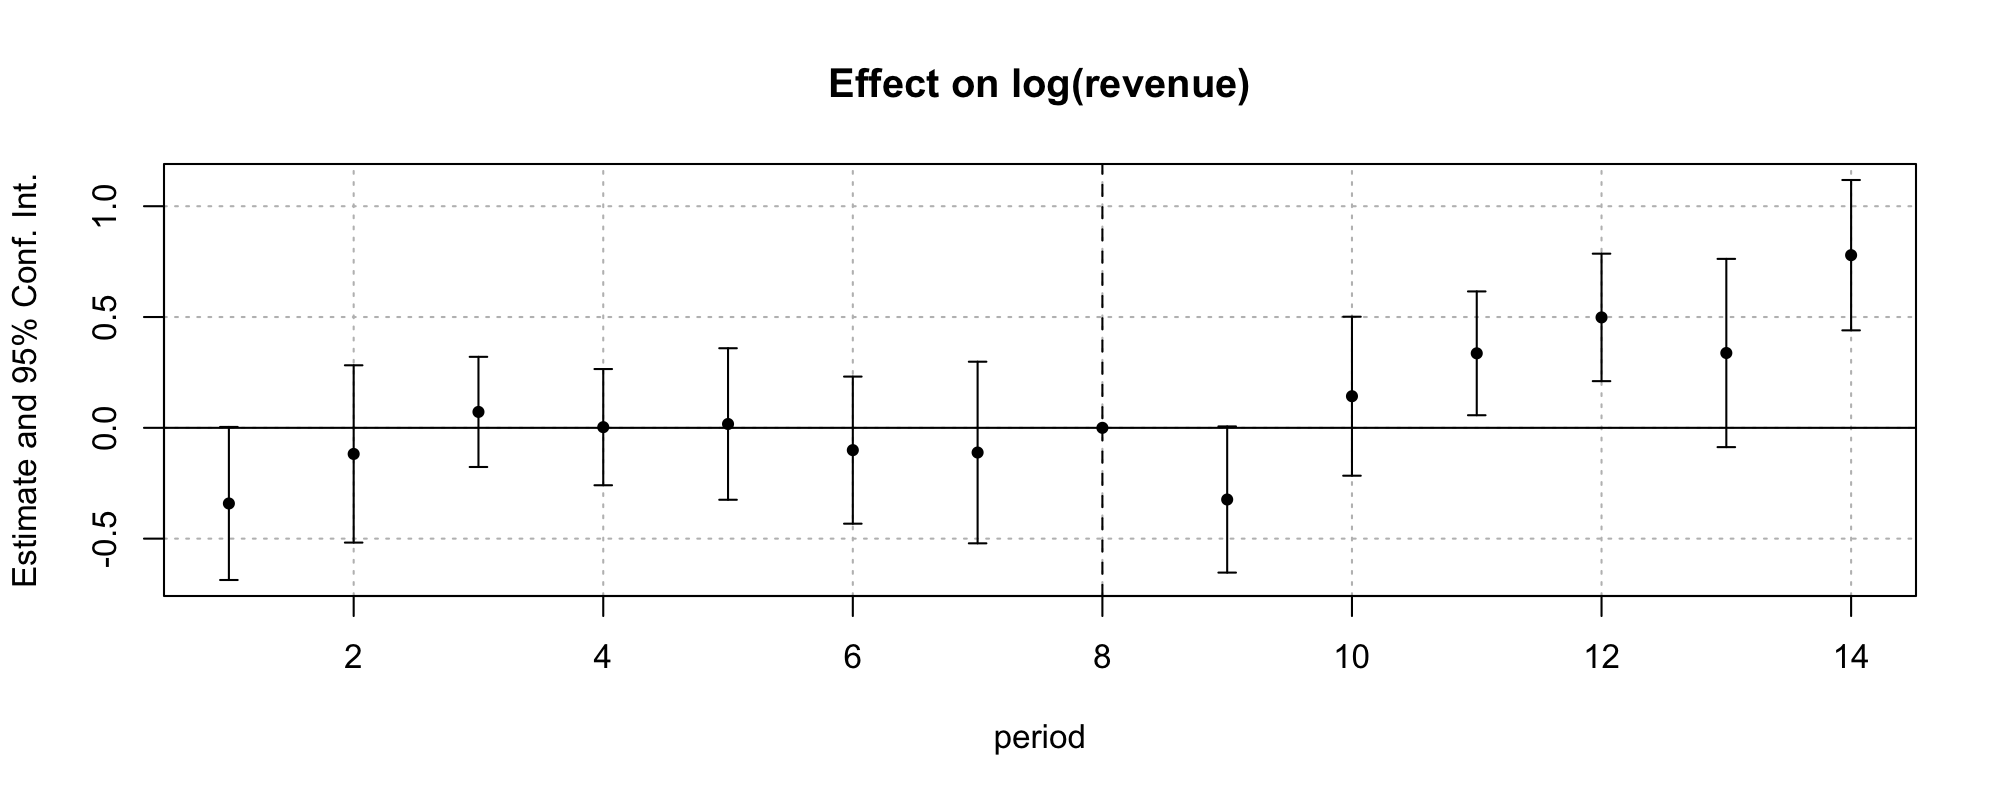}
% \vspace*{-3mm}
\caption{Dynamic Treatment Effect Plots of Generative AI on Market Equilibrium.}
\label{fig:event}
\vspace*{+10mm}
\end{figure}

\subsubsection{Placebo Test}
We conduct a placebo test using a fake treatment date. We use the data from January 2022 to August 2022, with the treatment assumed to have occurred in April 2022. We then estimate the same difference-in-differences specification in Equation (1). If no significant effects were found with this fake treatment date, it was concluded that the parallel trend assumption was not violated.
% We conduct a placebo test using a fake treatment date. We use the data from January 2022 to August 2022 and pretend that the treatment was in April 2022. We then estimate the same difference-in-differences specification in Equation (1). If we do not find significant effects with this fake treatment date, then the parallel trend assumption is not violated.

Table~\ref{tab:placebo_fake} depicts the estimated outcomes of the placebo test, and Table~\ref{tab:placebo_real} shows its comparison using the real treatment date. The results indicate that the effects of the placebo test are not statistically significant (at the 5\% level) and their magnitude is also much weaker than the real effects. This suggests that there are no differences between the treatment and control groups in the pretreatment periods, which supports the parallel trend assumption.
% Table~\ref{tab:placebo_fake} shows the estimates of the placebo test, and Table~\ref{tab:placebo_real} shows its comparison using the real treatment date. The results show that the effects of the placebo test are not significant (at the 5\% level) and their magnitude is also much weaker than the real effects, suggesting that there are no differences between the treatment and control groups in the pretreatment periods, which supports the parallel trend assumption.

\begin{table*}[h!]
% \linespread{1}
% \huge
% \selectfont
% \footnotesize
\centering
    % \vspace{-5mm}
    \resizebox{\linewidth}{!}{
   \begin{tabular}{lcccccc}
      \tabularnewline \midrule \midrule
      Dependent Variables:    & price                 & volume   & revenue & log(price)            & log(volume)  & log(revenue)\\  
      Model:                  & (1)                   & (2)      & (3)     & (4)                   & (5)          & (6)\\  
      \midrule
      \emph{Variables}\\
      treated $\times$ after  & -22.62                & 0.5474   & 399.3   & -0.0112               & 0.1311$^{*}$ & 0.1199\\   
                              & (106.7)               & (0.5632) & (910.9) & (0.0740)              & (0.0688)     & (0.1055)\\   
      \midrule
      \emph{Fixed-effects}\\
      art\_category           & Yes                   & Yes      & Yes     & Yes                   & Yes          & Yes\\  
      year\_week              & Yes                   & Yes      & Yes     & Yes                   & Yes          & Yes\\  
      \midrule
      \emph{Fit statistics}\\
      Observations            & 716                   & 716      & 716     & 716                   & 716          & 716\\  
      R$^2$                   & 0.41401               & 0.63994  & 0.22616 & 0.55645               & 0.61816      & 0.30111\\  
      Within R$^2$            & $7.75\times 10^{-5}$  & 0.00186  & 0.00034 & $3.32\times 10^{-5}$  & 0.00726      & 0.00227\\  
      \midrule \midrule
      \multicolumn{7}{l}{\emph{Clustered (lastdigit) standard-errors in parentheses}}\\
      \multicolumn{7}{l}{\emph{Signif. Codes: ***: 0.01, **: 0.05, *: 0.1}}\\

   \end{tabular}  
   }

% \vspace{+5mm}
\caption{The Impact of Generative AI on Market Equilibrium - Placebo Test}
\label{tab:placebo_fake}
\end{table*}

\begin{table*}[h!]
% \linespread{1}
% \huge
% \selectfont
% \footnotesize
\centering
    % \vspace{-5mm}
    \resizebox{\linewidth}{!}{
   \begin{tabular}{lcccccc}
      \tabularnewline \midrule \midrule
      Dependent Variables:    & price          & volume        & revenue         & log(price)      & log(volume)   & log(revenue)\\  
      Model:                  & (1)            & (2)           & (3)             & (4)             & (5)           & (6)\\  
      \midrule
      \emph{Variables}\\
      treated $\times$ after  & -656.6$^{***}$ & 14.06$^{***}$ & 5,702.6$^{***}$ & -0.5630$^{***}$ & 1.249$^{***}$ & 0.6864$^{***}$\\   
                              & (48.88)        & (0.3398)      & (654.3)         & (0.0507)        & (0.0412)      & (0.0692)\\   
      \midrule
      \emph{Fixed-effects}\\
      art\_category           & Yes            & Yes           & Yes             & Yes             & Yes           & Yes\\  
      year\_week              & Yes            & Yes           & Yes             & Yes             & Yes           & Yes\\  
      \midrule
      \emph{Fit statistics}\\
      Observations            & 1,253          & 1,253         & 1,253           & 1,253           & 1,253         & 1,253\\  
      R$^2$                   & 0.41023        & 0.65433       & 0.34534         & 0.48933         & 0.66103       & 0.39564\\  
      Within R$^2$            & 0.08167        & 0.45615       & 0.05610         & 0.07988         & 0.41087       & 0.07020\\  
      \midrule \midrule
      \multicolumn{7}{l}{\emph{Clustered (lastdigit) standard-errors in parentheses}}\\
      \multicolumn{7}{l}{\emph{Signif. Codes: ***: 0.01, **: 0.05, *: 0.1}}\\

   \end{tabular}  
   }

% \vspace{+5mm}
\caption{The Impact of Generative AI on Market Equilibrium - Real Treatment Date}
\label{tab:placebo_real}
\end{table*}

\subsection{Completed Order Results} \label{app:complete}
In this study, we utilize data from all orders, including both completed and uncompleted orders, to compute market equilibrium. In this section, we present the results obtained from the analysis of only the data from all completed orders.

Table~\ref{tab:completed} presents the results obtained using the completed order data\footnote{Columns (4) through (6) in Table~\ref{tab:completed} are the same as columns (1) through (3) in Table~\ref{tab:reg_supply}, as we used them for the supplier analysis.}. The estimators in Table~\ref{tab:completed} are in close alignment with, and even more promising than, the estimators in Table~\ref{tab:reg_main} using data from all orders, suggesting that our results are robust to whether we use all orders or only completed orders. One straightforward explanation is that customers make the order decision and set the price according to the status of current orders listed on the focal platform.
% Table~\ref{tab:completed} reports the results using the completed order data\footnote{Columns (4) through (6) in Table~\ref{tab:completed} are the same as columns (1) through (3) in Table~\ref{tab:reg_supply}, as we used them for the supplier analysis.}. The estimators in Table~\ref{tab:completed} are very close to, and even more promising than, the estimators in Table~\ref{tab:reg_main} using data from all orders, suggesting that our results are robust to whether we use all orders or only completed orders. A straightforward explanation is that customers make the order decision and set the price according to the status of current orders listed on the focal platform.

\begin{table*}[!t]
% \linespread{1}
% \huge
% \selectfont
% \footnotesize
\centering
    % \vspace{-5mm}
    \resizebox{\linewidth}{!}{
   \begin{tabular}{lcccccc}
      \tabularnewline \midrule \midrule
      Dependent Variables:    & price                    & volume                   & revenue                 & log(price)               & log(volume)              & log(revenue)\\  
      Model:                  & (1)                      & (2)                      & (3)                      & (4)                      & (5)                      & (6)\\  
      \midrule
      \emph{Variables}\\
      treated $\times$ after  & -502.4$^{***}$           & 45.77$^{***}$            & 23,375.2$^{***}$         & -0.4915$^{***}$          & 1.171$^{***}$            & 0.6790$^{***}$\\   
                              & ($1.59\times 10^{-12}$)  & ($1.17\times 10^{-13}$)  & ($7.54\times 10^{-11}$)  & ($1.33\times 10^{-15}$)  & ($3.51\times 10^{-15}$)  & ($2.02\times 10^{-15}$)\\    
      \midrule
      \emph{Fixed-effects}\\
      art\_category           & Yes                      & Yes                      & Yes                      & Yes                      & Yes                      & Yes\\  
      year\_week              & Yes                      & Yes                      & Yes                      & Yes                      & Yes                      & Yes\\  
      \midrule
      \emph{Fit statistics}\\
      Observations            & 126                      & 126                      & 126                      & 126                      & 126                      & 126\\  
      R$^2$                   & 0.77403                  & 0.85943                  & 0.73179                  & 0.79706                  & 0.89378                  & 0.73652\\  
      Within R$^2$            & 0.22630                  & 0.72652                  & 0.24330                  & 0.21484                  & 0.67848                  & 0.19868\\  
      \midrule \midrule
      \multicolumn{7}{l}{\emph{Clustered (art\_category) standard-errors in parentheses}}\\
      \multicolumn{7}{l}{\emph{Signif. Codes: ***: 0.01, **: 0.05, *: 0.1}}\\

   \end{tabular}  
   }

% \vspace{+5mm}
\caption{The Impact of Generative AI on Market Equilibrium - Completed Order Results}
\label{tab:completed}
\end{table*}

\begin{table*}[h!]
% \linespread{1}
% \huge
% \selectfont
% \footnotesize
\centering
    % \vspace{-5mm}
    \resizebox{\linewidth}{!}{
   \begin{tabular}{lcccccccc}
      \tabularnewline \midrule \midrule

      Dependent Variables:    & log(price\_upper)        & log(revenue\_upper)      & log(price\_middle)       & log(revenue\_middle)  & log(price\_ul)           & log(revenue\_ul)         & log(price\_lu)           & log(revenue\_lu)\\   
      Model:                  & (1)                      & (2)                      & (3)                      & (4)                   & (5)                      & (6)                      & (7)                      & (8)\\  
      \midrule
      \emph{Variables}\\
      treated $\times$ after  & -0.5168$^{***}$          & 0.6940$^{***}$           & -0.5564$^{***}$          & 0.6544$^{***}$        & -0.3046$^{***}$          & 0.9062$^{***}$           & -0.8558$^{***}$          & 0.3549$^{***}$\\   
                              & ($1.71\times 10^{-15}$)  & ($1.39\times 10^{-15}$)  & ($1.43\times 10^{-15}$)  & ($2\times 10^{-15}$)  & ($7.52\times 10^{-16}$)  & ($2.74\times 10^{-15}$)  & ($2.16\times 10^{-15}$)  & ($1.35\times 10^{-15}$)\\    
      \midrule
      \emph{Fixed-effects}\\
      art\_category           & Yes                      & Yes                      & Yes                      & Yes                   & Yes                      & Yes                      & Yes                      & Yes\\  
      year\_week              & Yes                      & Yes                      & Yes                      & Yes                   & Yes                      & Yes                      & Yes                      & Yes\\  
      \midrule
      \emph{Fit statistics}\\
      Observations            & 126                      & 126                      & 126                      & 126                   & 126                      & 126                      & 126                      & 126\\  
      R$^2$                   & 0.84131                  & 0.84148                  & 0.87004                  & 0.85222               & 0.95451                  & 0.92018                  & 0.95013                  & 0.94098\\  
      Within R$^2$            & 0.42816                  & 0.44333                  & 0.47405                  & 0.42184               & 0.20118                  & 0.58389                  & 0.67316                  & 0.17232\\  
      \midrule \midrule
      \multicolumn{9}{l}{\emph{Clustered (art\_category) standard-errors in parentheses}}\\
      \multicolumn{9}{l}{\emph{Signif. Codes: ***: 0.01, **: 0.05, *: 0.1}}\\

   \end{tabular}  
   }

% \vspace{+5mm}
\caption{The Impact of Generative AI on Market Equilibrium - Alternative Price Measurements}
\label{tab:reg_alterprice}
\end{table*}

\subsection{Alternative Price Measurements} \label{app:price}
In consideration of privacy concerns, it is not feasible to obtain the precise price of each order. Consequently, the average price and overall revenue are calculated based on the lower bound of the price range set by consumers, as this may more accurately reflect the consumers' genuine willingness to accept their orders than the upper bound. 
% Due to privacy concerns, we cannot obtain the exact price of each order. As a result, we calculate the average price and overall revenue based on the lower bound of the price range set by consumers because the lower bound may better reflect the true willingness of consumers to accept their orders than the upper bound. 

In this section, we test the alternative price measurements. $price\_upper$ and $revenue\_upper$ use the upper bound of the price range. $price\_middle$ and $revenue\_middle$ use the mean of the lower and upper bounds. Additionally, the most extreme cases are constructed using the lower bound for orders prior to the leak and the upper bound for orders subsequent to the leak, resulting in $price\_lu$ and $revenue\_lu$. Similarly, the values of $price\_ul$ and $revenue\_ul$ are obtained using the upper bound prior to and the lower bound subsequent to the leak.

% In this section, we test the alternative price measurements. $price\_upper$ and $revenue\_upper$ use the upper bound of the price range. $price\_middle$ and $revenue\_middle$ use the mean of the lower and upper bounds. We also construct the most extreme cases, using the lower bound for orders before the leak and the upper bound for orders after the leak, and get $price\_lu$ and $revenue\_lu$. We also get $price\_ul$ and $revenue\_ul$ using the upper bound before and the lower bound after.

Table~\ref{tab:reg_alterprice} demonstrates the robustness of our results across different price measures. In particular, the estimates in columns (1) through (4) of Table~\ref{tab:reg_alterprice} are similar to the corresponding estimates in Table~\ref{tab:reg_main}, indicating that generative AI reduces average prices and increases total revenues. Furthermore, the estimates in columns (5) through (8) are of the same magnitude, suggesting that our results hold even in the most extreme cases.

This is due to the fact that the theoretical analysis of market equilibrium ensures that prices will invariably decline. Furthermore, the rise in overall revenue is attributable to the surge in order volume, which is not contingent on the manner in which price is measured.
% This is because the theoretical analysis of market equilibrium guarantees that prices will always fall. In addition, the increase in overall revenue is driven by the boost in order volume, which is independent of how we measure price.

\subsection{Longer Time Period} \label{app:period}
To investigate the longevity of the effects of generative AI, we have extended the post-treatment period from five months to twelve months. Our data sample encompasses the period from January 2022 to September 2023.
% We extend the post-treatment period from five months to twelve months to examine the extent to which the effects of generative AI persist over time, constructing a data sample from January 2022 to September 2023.

For causal inference reasons, we prefer to use a relatively brief period of time, as this ensures an ideal scenario in which generative AI exerts an influence on the "tachie" market, yet does not affect the "wallpaper" market, due to the specifications of NovelAI. A longer period may yield underestimated results due to the emergence of new generative AI for wallpaper. Hopefully, Table~\ref{tab:longer} shows that the average price decreases more (-81\%) and the order volume (155\%) and overall revenue increase more (73\%) in the longer period, suggesting that the impact of generative AI is not only persistent but also strengthened in the long run.
% For causal inference reasons, we prefer to use a short period because it ensures an ideal scenario where generative AI affects the "tachie" market but not the "wallpaper" market due to NovelAI's specification. In a longer period, it is likely that new generative AI has been developed for wallpaper, leading to an underestimated result. Hopefully, Table~\ref{tab:longer} shows that the average price decreases more (-81\%) and the order volume (155\%) and overall revenue increase more (73\%) in the longer period, suggesting that the impact of generative AI is not only persistent but also strengthened in the long run.

\begin{table*}[h!]
% \linespread{1}
% \huge
% \selectfont
% \footnotesize
\centering
    % \vspace{-5mm}
    \resizebox{\linewidth}{!}{
   \begin{tabular}{lcccccc}
      \tabularnewline \midrule \midrule
      Dependent Variables:    & price                    & volume                   & revenue                 & log(price)               & log(volume)              & log(revenue)\\  
      Model:                  & (1)                      & (2)                      & (3)                      & (4)                      & (5)                      & (6)\\  
      \midrule
      \emph{Variables}\\
      treated $\times$ after  & -772.9$^{***}$           & 177.1$^{***}$            & 56,384.1$^{***}$         & -0.8181$^{***}$          & 1.550$^{***}$            & 0.7318$^{***}$\\   
                              & ($5.14\times 10^{-12}$)  & ($1.17\times 10^{-12}$)  & ($3.87\times 10^{-10}$)  & ($5.14\times 10^{-15}$)  & ($8.55\times 10^{-15}$)  & ($4.62\times 10^{-15}$)\\    
      \midrule
      \emph{Fixed-effects}\\
      art\_category           & Yes                      & Yes                      & Yes                      & Yes                      & Yes                      & Yes\\  
      year\_week              & Yes                      & Yes                      & Yes                      & Yes                      & Yes                      & Yes\\  
      \midrule
      \emph{Fit statistics}\\
      Observations            & 186                      & 186                      & 186                      & 186                      & 186                      & 186\\  
      R$^2$                   & 0.86955                  & 0.88528                  & 0.87977                  & 0.87633                  & 0.89432                  & 0.89620\\  
      Within R$^2$            & 0.63660                  & 0.82983                  & 0.43064                  & 0.63307                  & 0.83147                  & 0.48623\\  
      \midrule \midrule
      \multicolumn{7}{l}{\emph{Clustered (art\_category) standard-errors in parentheses}}\\
      \multicolumn{7}{l}{\emph{Signif. Codes: ***: 0.01, **: 0.05, *: 0.1}}\\

   \end{tabular}  
   }

% \vspace{+5mm}
\caption{The Impact of Generative AI on Market Equilibrium - Longer Time Period}
\label{tab:longer}
\end{table*}
